# Supplementary material for: BabyLMs for isiXhosa: Data-Efficient Language Modelling in a Low-Resource Context
Source: arXiv:2501.03855 source file (2025-01-07)
Supplement: Supplementary file 1 [file appendix.tex]

\section{Appendix}
\label{sec:appendix}

The \textbf{RoBERTa} model uses a simple BPE (Byte Pair Encoding) tokenizer. We adopt the original hyperparameters from the RoBERTa library, which are specified in \autoref{Table1}. The model was trained from scratch on 200 epochs of the above isiXhosa dataset in order to produce a suitable baseline.

For \textbf{ELC-BERT}, we make use of the original
architectural hyperparameters used by its authors in their original submission to the Strict-Small track in the BabyLM challenge – 12 hidden layers with 6 attention heads and a feed-forward hidden size of 1024. The model pre-tokenizes text using ByteLevel and Digits processing, and employs a WordPiece model for the main tokenization. Due to computational constraints, we train our model for 200 epochs, instead of the 2000 epoch regimen used by the original authors. We adapt our learning rate to 5e-4 and batch size to 128, as the parameters used in the authors original submission (batch size of 256 and learning rate of $1e^{-2}$) perform sub-optimally on our adapted training regimen \cite{georges-gabriel-charpentier-samuel-2023-layers}.

The initial phase of training the \textbf{MLSM} model involved setting up a Teacher model using the WURA dataset to evaluate the MLSM model’s effectiveness with all its components trained from scratch, minimizing the influence of external pretraining methods. The Teacher model employed a BERT-base-cased architecture using standard MLM training with the hyperparameters in \autoref{Table1}. These were selected based on their success in training the Teacher model for the BabyLM 10 million track challenge, suggesting they are well-suited for our dataset of 13 million words. Next, a Tokenizer was set up for the Student model which matched the Teacher model's Tokenizer except with \( k = 3000 \) added tokens in the format [MASK-n] with n ranging from 0 to 2999. Subsequently, a Semantic Dictionary was set up using one of the Teacher model's hidden layers using modified code from the MLSM repository. For this project, \( k \) was set to 3000 and \( \lambda \) was set to 0.05, matching the hyperparameters used by the BabyLM MLSM model, as they found these to be the most efficient parameters on the 10 million word dataset \cite{berend2023}.  Finally, the student model was trained for 200 epochs on a BERT-base-cased architecture with a batch size of 64 and a learning rate of 1e-4 as detailed in Table \ref{Table1}.

\begin{table}[htbp]
\centering
\caption{NLU test results averaged across 5 runs, comparing baseline to BabyLM models to skyline models RoBERTa and to MLSM. For NER and news topic classification we report weighted f1 scores, whilst for POS tagging we report accuracy. We omit standard deviations for our models here for clarity, but attach them to the appendix table at the end of the report.}
\label{tab:nlu-results}
\begin{tabular}{llccc}
\hline
Task & Epochs & RoBERTa & ELC-BERT & MLSM \\
\hline\hline
NER  & 20     & 80.8 & \underline{86.6} & 85.6 \\
     & 100    & 85.1 & \underline{\textbf{88.7}} & 86.6 \\
     & 200    & 85.4 & \underline{88.6} & 87.0 \\
\hline
NEWS & 20     & 93.0 & 89.7 & \underline{95.2} \\
     & 100    & \underline{96.5} & 93.4 & 95.2 \\
     & 200    & \underline{\textbf{97.6}} & 95.0 & 95.4 \\
\hline
POS  & 20     & 84.4 & \underline{\textbf{88.0}} & 87.0 \\
     & 100    & 87.0 & \underline{87.9} & 87.5 \\
     & 200    & 87.0 & \underline{87.7} & 87.4 \\
\hline\hline
\multicolumn{5}{l}{Skyline Models:} \\
\hline\hline
Task & & XLM-R & Afro-XLMR & Nguni-XLMR \\
\hline
NER  &        & 88.1 & 89.9 & \textbf{90.4} \\
NEWS &        & 89.2 & 97.3 & \textbf{98.2} \\
POS  &        & 88.1 & 88.7 & \textbf{88.3} \\
\hline\hline
\end{tabular}
\end{table}

\subsection{Training efficiency}

\begin{table}[htbp]
\centering
\caption{Approximate training time to reach checkpoints on a single V100 GPU in hours, rounded to the nearest hour}
\label{tab:elc-bert-epochs}
\begin{tabular}{lcccc}
\hline
Model & 20 epochs & 100 epochs & 200 epochs\\
\hline
RoBERTa  & 12 & 60 & 120 \\
ELC-BERT & 3 & 13 & 26 \\
MLSM  & 9 & 44 & 88 \\
\hline
\end{tabular}
\end{table}

\begin{table}[htbp]
\centering
\caption{NLU test results with standard deviations averaged across 5 runs. Standard deviations are shown after the $\pm$ sign where available. We include standard deviations for our models we run ourselves, but omit it for models that do not report it.}
\label{tab:nlu-results}
\begin{tabular}{llccc}
\hline
Task & Epochs & RoBERTa & ELC-BERT & MLSM \\
\hline\hline
NER  & 20     & 80.8 $\pm$ 0.7 & \underline{86.6} $\pm$ 0.4 & 84.6 $\pm$ 0.3 \\
     & 100    & 85.1 $\pm$ 0.3 & \underline{\textbf{88.7}} $\pm$ 0.5 & 86.6 $\pm$ 0.4 \\
     & 200    & 85.4 $\pm$ 0.4 & \underline{88.6} $\pm$ 0.6 & 87.0 $\pm$ 0.4 \\
\hline
NEWS & 20     & 93.0 $\pm$ 0.5 & 89.7 $\pm$ 0.8 & \underline{94.5} $\pm$ 1.0 \\
     & 100    & \underline{96.5} $\pm$ 0.2 & 93.4 $\pm$ 0.9 & 95.2 $\pm$ 0.6 \\
     & 200    & \underline{\textbf{97.6}} $\pm$ 0.5 & 95.0 $\pm$ 0.5 & 95.4 $\pm$ 0.2 \\
\hline
POS  & 20     & 84.4 $\pm$ 0.2 & \underline{\textbf{88.0}} $\pm$ 0.1 & 85.5 $\pm$ 0.1 \\
     & 100    & 87.0 $\pm$ 0.1 & \underline{87.9} $\pm$ 0.2 & 87.5 $\pm$ 0.1 \\
     & 200    & 87.0 $\pm$ 0.1 & \underline{87.7} $\pm$ 0.3 & 87.4 $\pm$ 0.1 \\
\hline\hline
\multicolumn{5}{l}{Skyline Models:} \\
\hline\hline
Task & & XLM-R & Afro-XLMR & Nguni-XLMR \\
\hline
NER  &        & 88.1 & 89.9 & \textbf{90.4} $\pm$ 0.004 \\
NEWS &        & 89.2 & 97.3 & \textbf{98.2} $\pm$ 0.5 \\
POS  &        & 88.1 & 88.7 & \textbf{88.3} $\pm$ 0.1 \\
\hline\hline
\end{tabular}
\end{table}
